# Supplementary material for: Online Time Series Anomaly Detection with State Space Gaussian Processes
Source: arXiv:2201.06763 source file (2022-01-18)
Supplement: Supplementary file 1 [file appendix.pdf]

## 595 A GPFA

### 596 A.1 Unidentifiability of $C$ in Factor Analysis

597 It is known that Factor Analysis is not identifiable: multiple solutions provide the same optimal  
 598 likelihood. Let  $Q$  to be an arbitrary orthogonal rotation matrix of size  $K \times K$  satisfying  $QQ^T = I$ .  
 599 We can obtain a different loading matrix  $\tilde{C} = CQ$  for which the likelihood is given by:

$$p(\mathbf{y}_{:,t}|\theta) = \mathcal{N}(\mathbf{y}_{:,t}|\mathbf{d}, \Psi + \tilde{C}\tilde{C}^T) \quad (13)$$

$$= \mathcal{N}(\mathbf{y}_{:,t}|\mathbf{d}, \Psi + CQQ^TC^T) \quad (14)$$

$$= \mathcal{N}(\mathbf{y}_{:,t}|\mathbf{d}, \Psi + CC^T) \quad (15)$$

### 600 A.2 Closed form model parameter updates

601 Using  $q(\mathbf{z}_{:,t}) = \mathcal{N}(\mathbf{z}_{:,t}|\boldsymbol{\mu}_t, \Sigma_t)$ , the posterior distribution on the latent at each time step  $t$  inferred in  
 602 the E-step, we obtain the closed form updates for the model parameters:

$$\begin{aligned} C^* &= \left( \sum_{t=1}^T (\mathbf{y}_{:,t} - \mathbf{d}) \boldsymbol{\mu}_t^T \right) \left( \sum_{t=1}^T (\Sigma_t + \boldsymbol{\mu}_t \boldsymbol{\mu}_t^T) \right)^{-1} \\ \mathbf{d}^* &= \frac{1}{T} \sum_{t=1}^T (\mathbf{y}_t - C \boldsymbol{\mu}_t) \\ \Psi &= \frac{1}{T} \sum_{t=1}^T ((\mathbf{y}_t - C \boldsymbol{\mu}_t - \mathbf{d})(\mathbf{y}_t - C \boldsymbol{\mu}_t - \mathbf{d})^T + C \Sigma_t C^T) \end{aligned}$$

603 These are the model parameters that maximise the evidence lower bound in the M-step. Note that the  
 604 derivations and updates are the same as for Factor Analysis.

## 605 B Robust filtering algorithm

---

### Algorithm 1: Robust Kalman filtering

---

**Input:** Time series  $\mathbf{t} = (\mathbf{y}_t)_{t=1}^T$ , update threshold  $\rho$

```

1  $o := 1$  // Index last relevant observation
2 for  $t \in \{1, \dots, T\}$  do
3    $\Delta_t \leftarrow t - o$ 
4    $\mathbf{A}_t = \exp(\mathbf{F} \Delta_t)$ 
5    $\mathbf{Q}_t = \mathbf{P}_\infty - \mathbf{A}_t \mathbf{P}_\infty \mathbf{A}_t^T$ 
   // Kalman prediction
6    $\mathbf{m}_{t|t-1}, \mathbf{P}_{t|t-1} \leftarrow$  prediction with Eq. 4
7    $\log\{p(\mathbf{y}_t)\} \leftarrow$  likelihood of observed with Eq. 5
   // Robustify
8   if  $\log p(\mathbf{y}_t) > \rho$  then
9      $\mathbf{m}_{\text{flt}}, \mathbf{P}_{\text{flt}} \leftarrow$  filtering mean and covariance
10     $o \leftarrow t$  // set o to last normal index;
11 end
```

---

## 606 C Computational and memory complexity

607 GPs are known to scale very poorly to big datasets but the combination of introduced methods allows  
 608 for lightweight training and inference. Recall that  $D$  is the number of observed dimensions,  $K$  the  
 609 number of latent processes, and  $T$  the number of training time steps. We denote  $L$  as the maximum  
 610 state space dimension among all latent processes.

611 The computational complexity for **training** is  $\mathcal{O}(TD^3KL^2 + TKL^3)$  when we constrain the columns  
 612 of  $\mathbf{C}$  to be orthogonal and  $\mathcal{O}(TD^3K^2L^2 + TK^3L^3)$  without constraints. In both cases it is linear in  
 613 the number of training points. When dealing with very high dimensional time series and few latent  
 614 processes, one can map the input to a  $K$  dimensional space proposed by [4] to allow the training  
 615 complexity to scale linearly in  $D$  but cubically in  $K$ .

616 **Inference** requires the computation of the likelihood of the observation and the Kalman update.  
 617 The computations complexity is  $\mathcal{O}(D^3KL^2 + KL^3)$  if  $\mathbf{C}$  is constrained as orthogonal otherwise  
 618  $\mathcal{O}(D^3K^2L^2 + K^3L^3)$  without constraints. Beyond making the complexity scale linearly in the  
 619 number of latent dimensions, the orthogonalisation of  $\mathbf{C}$  allows to compute the filtering and smoothing  
 620 (and the E-step) for each of the latent process independently of each other. In such setting, it can be  
 621 easily parallelized only with only little sequential calculation.

## 622 D Experiments

### 623 D.1 State-Space Matrices

624 In this section, we exemplify the state space representation of the Matérn Kernel with  $\nu = \frac{3}{2}$ . For  
 625 a more comprehensive enumeration of other covariance functions, we refer the interested reader  
 626 to Solin [41]. In the following example,  $\mathbf{F}$  is the feedback matrix of the corresponding SDE,  $\mathbf{h}^T$  its  
 627 measurement model,  $\mathbf{P}_\infty$  the stationary state covariance matrix (i.e. the state the process stabilises to  
 628 in infinity), and  $\mathbf{A}$  the *discrete-time* state transition matrix.

629 State-space matrices for Matern32-kernel with length-scale  $l$ , variance  $\sigma^2$  and let  $\lambda = \frac{\sqrt{3}}{l}$ :

$$\mathbf{F} = \begin{bmatrix} 0 & 1 \\ -\lambda^2 & -2\lambda \end{bmatrix}, \quad \mathbf{h}^T = [1 \quad 0], \quad \mathbf{P}_\infty = \begin{bmatrix} \sigma^2 & 0 \\ 0 & \lambda^2 \sigma^2 \end{bmatrix},$$

$$\mathbf{A} = \exp(\mathbf{F}\Delta_t)$$

630 Furthermore, it was shown [41, 39, 42] that the addition and multiplication of covariance functions in  
 631 state space can be expressed in terms of block diagonals and Kronecker products ( $\otimes$ ) and sums ( $\oplus$ )  
 632 as shown below.

633 **Kernel Addition** The addition of two kernels  $K_1$  and  $K_2$  in the state space formulation is defined  
 634 by stacking their respective state-space matrices:

$$\mathbf{F} = \text{blkdiag}(\mathbf{F}_1, \mathbf{F}_2), \quad \mathbf{H} = \text{blkdiag}(\mathbf{H}_1, \mathbf{H}_2),$$

$$\mathbf{P}_\infty = \text{blkdiag}(\mathbf{P}_{\infty 1}, \mathbf{P}_{\infty 2}), \quad \mathbf{A} = \exp(\mathbf{F}\Delta_t)$$

635 **Kernel Multiplication** The multiplication of two kernels  $K_1$  and  $K_2$  in the state space formulation  
 636 is defined by the Kronecker sum of the respective feedback matrices and the Kronecker product of  
 637 the remaining state matrices:

$$\mathbf{F} = \mathbf{F}_1 \oplus \mathbf{F}_2, \quad \mathbf{H} = \mathbf{H}_1 \otimes \mathbf{H}_2,$$

$$\mathbf{P}_\infty = \mathbf{P}_{\infty 1} \otimes \mathbf{P}_{\infty 2}, \quad \mathbf{A} = \exp(\mathbf{F}\Delta_t)$$

### 638 D.2 Implementation Details

639 **RRCF** The RRCF algorithm represents a predefined number of observations (i.e. shingle size) as a  
 640 higher-dimensional point. In a streaming scenario each new observation gives rise to a new shingle  
 641 which is used to update the random cut forest. Using reservoir sampling, the tree can be updated in  
 642 sublinear time which makes this approach particularly attractive for the online setting. The authors  
 643 define the collusive displacement score (CODISP), a measure of change in model complexity when a

new observation is inserted, as their anomaly score. We run RRCF with 40 trees of size 256 and a shingle size of 4.

As for the selected kernel for ssGP, we do not perform a kernel search, but instead choose a versatile Kernel consisting of the addition of a Brownian motion-kernel with a multiplication of a Matern32 and a Cosine-kernel. For ssGPFA, we use four independent ssGPs with fixed Matern32-kernels with lengthscales (130, 200, 50, 10). That being said, our method can readily be used for sophisticated Kernel search algorithms such as [29].

For all methods, we fix the robustification threshold  $\rho$  to be  $1e-12$  without performing any parameter search. We use the L-BFGS-B [6] algorithm to fit our models for maximally 20 epochs.

### D.3 Synthetic Data

The data generating process yielding the time series of Figure 2 is defined by the following equation.

$$f(t) = \cos(0.04t + 0.33\pi) \cdot \sin(0.2t) + \epsilon_{\text{synth.}} + 5/300t, \quad (16)$$

with  $\epsilon_{\text{synth.}} \sim \mathcal{N}(0, 0.15)$ .

## E Data Sets

Table 3 shows data statistics on the used benchmark data sets.  $\bar{n}$  refers to the mean time series length.

Table 3: Statistics for the used benchmark data sets. The fraction of anomalies refers to point anomalies, not to anomaly ranges.

| Data Set | Sub Data Set          | Num. TS | $D$ | $\bar{n}$ (train/test) | % Anomalies |
|----------|-----------------------|---------|-----|------------------------|-------------|
| NAB      | realAWSCloudwatch     | 17      | 1   | 3984                   | 9.3%        |
|          | realAdExchange        | 6       | 1   | 1601                   | 10.0%       |
|          | realKnownCause        | 7       | 1   | 9937                   | 9.6%        |
|          | realTraffic           | 7       | 1   | 2237                   | 10.0%       |
|          | realTweets            | 10      | 1   | 15863                  | 9.9%        |
|          | artificialWithAnomaly | 6       | 1   | 4032                   | 10.0%       |
| NASA     | SMAP                  | 54      | 25  | 2555/8070              | 12.83 %     |
|          | MSL                   | 27      | 55  | 1785/2730              | 10.53 %     |
| SMD      | machine-1             | 8       | 38  | 24296/24296            | 6.04 %      |
|          | machine-2             | 9       | 38  | 23691/24813            | 4.34 %      |
|          | machine-3             | 11      | 38  | 26424/26429            | 2.75 %      |

658
